# Supplementary material for: DiffH2O: Diffusion-Based Synthesis of Hand-Object Interactions from Textual Descriptions
Source: arXiv:2403.17827 source file (2024-12-23)
Supplement: Supplementary file 2 [file supp_tab_action_correctness_per_obj.tex]

\begin{table*}[]
  \centering
    \resizebox{0.8\textwidth}{!}{%
\begin{tabular}{@{}l|ll|ll|c|cccccccccc@{}}
\toprule
 & \multicolumn{2}{c|}{Split} & \multicolumn{2}{c|}{Textual input form} & \begin{tabular}[c]{@{}c@{}}Action\\ correctness\end{tabular} & \multicolumn{8}{c}{Action correctness over object classes} \\ \midrule
\multicolumn{1}{l|}{Method} & \multicolumn{1}{c}{Train split} & \multicolumn{1}{c|}{Test split} & \multicolumn{1}{c}{Train input} & \multicolumn{1}{c|}{Test input} & Overall & apple & mug & train & \begin{tabular}[c]{@{}c@{}}alarm\\ clock\end{tabular} & elephant & \begin{tabular}[c]{@{}c@{}}medium\\ cylinder\end{tabular} & \begin{tabular}[c]{@{}c@{}}small\\ pyramid\end{tabular} & \begin{tabular}[c]{@{}c@{}}large\\ torus\end{tabular} \\ \midrule
IMOS* & subject & object & simple & simple & 90.3 & 90.9 & 89.5 & 77.8 & \textbf{100} & 80.0 & \textbf{100} & 83.3 & \textbf{100} \\
Ours & subject & object & simple & simple & \textbf{99.5} & \textbf{100} & \textbf{97.4} & \textbf{100} & \textbf{100} & \textbf{100} & \textbf{100} & \textbf{100} & \textbf{100} \\
\midrule
Ours & object & object & \multicolumn{1}{c}{simple} & \multicolumn{1}{c}{simple} & 89.7 & 81.8 & 92.1 & 50.0 & 100 & 100 & 100 & 100 & 100 \\
\midrule
Ours & object & object & \multicolumn{1}{c}{simple} & comprehensive & 54.8 & 40.9 & 55.3 & 16.7 & 52.6 & 80.0 & 75 & 50.0 & 68.8 \\ 
Ours & object & object & comprehensive & comprehensive & 93.5 & 95.5 & 94.7 & 77.8 & 100 & 95.0 & 93.6 & 100 & 93.6 \\
\bottomrule
\end{tabular}
  }
 
\caption{\textbf{Details of the Text Evaluation.} Comparison of our method against IMoS and our model's variants that use different forms of textual input. We generate synthetic hand-object  pose sequences from each model based on textual prompts in two forms: a simple ("verb" + "object") and our detailed, proposed GRAB dataset annotations ("comprehensive"). We verify whether the generated sequences feature the correct action. We test all methods on our newly created unseen object split, which excludes 7 object classes for testing.} 
  \label{tab:action_correctness_per_obj}
\end{table*}
